# Supplementary material for: AcrossPlace: Do Vision--Language Models Recognize Places Beyond Their Source Views? A Comprehensive Benchmark
Source: arXiv:2611.15314 source file (2026-11-22)
Supplement: Supplementary file 1 [file X_suppl.tex]

% Extended descriptive analyses from frozen experiment artifacts.
\clearpage
\setcounter{page}{1}
\hypersetup{pageanchor=false}
\maketitlesupplementary
\appendix
\setcounter{table}{0}
\renewcommand{\thetable}{A\arabic{table}}
\newsavebox{\suppcontentbox}
\sbox{\suppcontentbox}{%
\begin{minipage}[t]{\textwidth}
\section{Evaluation Units, Evidence Scope, and Reproducibility}

\paragraph{Purpose and evidence scope.}
These analyses decompose the recorded benchmark results without changing a split, checkpoint, fusion weight, or relevance label. Principal scores, validation histories, paired diagnostic outcomes, gallery-draw summaries, and human-review records are read from archived artifacts. The newly produced city, capture-metadata, caption-length, and complementarity breakdowns are post-hoc descriptive analyses. They are not additional independently held-out experiments, and no new training or GPU inference is performed. Three epochs equalize the nominal epoch budget, not wall-clock duration, parameter count, or optimization objective.

\paragraph{Different estimands require different denominators.}
Principal galleries rank individual target images or descriptions, allowing several same-place positives. Paired diagnostics instead select one caption and one observation per place. Gallery-scaling experiments further retain only 500 query places while adding negatives. Human T2I queries the full P1 image gallery, whereas human I2T uses a focal-caption replacement against one caption per place. These settings answer related questions, but their percentages cannot be substituted for one another.

{\centering\small
\captionsetup{type=table}\caption{Evaluation-unit ledger. Counts specify what is actually ranked or averaged.}
\begin{tabular}{@{}lp{9.2cm}@{}}\toprule
Analysis & Unit and scope \\ \midrule
Principal P0 & 1,362 test places; 2,724 target images; 3,798 descriptions. \\
Principal P1 & 8,509 test places; 17,014 target images; 23,369 descriptions. \\
Paired transfer & 1,349 P0 / 8,425 P1 places; one caption and one source/target observation per place. \\
Matched geography & Five 1,000-place gallery draws within each protocol and checkpoint. \\
Fixed-query scaling & 500 query places; nested candidate pools up to 1,349 P0 / 8,425 P1 places. \\
Rule-status matching & 7,735 raw paired places; 4,291 after type/source/length matching. \\
Human retrieval & 240 descriptions at 237 places; 120 valid and 120 uncertain; one reviewer. \\
Qualitative outcomes & Three cached model configurations, supervised seed 42; first target view for I2T. \\\bottomrule
\end{tabular}\par}

\paragraph{Uncertainty and reproducibility.}
Training-seed SD describes three independently fitted checkpoints. Gallery-draw SD describes candidate sampling conditional on a checkpoint. Paired place bootstraps hold model weights fixed and preserve source/target pairing. None of these becomes fifteen independent training runs by multiplying three seeds and five draws. The released analysis inputs are SHA256-indexed, and machine-readable tables accompany the figures. Human labels were not used to choose model weights or checkpoints. Because the audit is balanced by rule status and includes repeated places, its unweighted percentages describe the reviewed sample rather than dataset-wide error prevalence.

\end{minipage}}
\typeout{SUPPLEMENT-PANEL-1-HEIGHT: \the\dimexpr\ht\suppcontentbox+\dp\suppcontentbox\relax}
\noindent\makebox[\columnwidth][l]{\usebox{\suppcontentbox}}\par

\clearpage
\sbox{\suppcontentbox}{%
\begin{minipage}[t]{\textwidth}
\section{Supervision Gains Across Ranks and Protocols}

\paragraph{A backbone-matched comparison.}
We subtract each frozen backbone's coarse score from its corresponding supervised recipe. CLIP uses the B/16 control; both SigLIP2 recipes use the same pretrained SigLIP2 control. These differences describe the combined effect of the recorded adaptation recipe and training exposure, not an isolated causal effect of the loss function. Encoder updates, heads, optimizer choices, and objectives differ across recipes.

\begin{center}
\includegraphics[width=.83\linewidth]{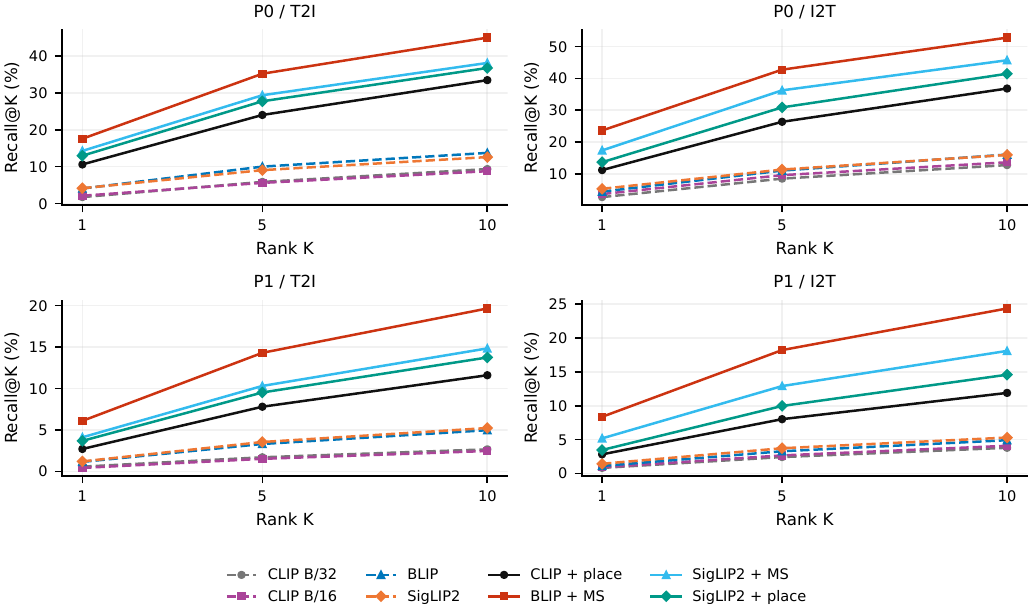}
\captionsetup{type=figure}
\caption{Principal full-gallery coarse recall at measured ranks 1, 5, and 10. Lines are visual guides; no intermediate ranks are inferred.}
\end{center}

{\centering\small
\setlength{\tabcolsep}{4pt}
\captionsetup{type=table}
\caption{Absolute gain over the matching pretrained backbone, in percentage points. Three-seed supervised means are compared with one frozen pretrained reference.}
\begin{tabular}{@{}llrrrr@{}}
\toprule
Protocol & Adaptation & \multicolumn{2}{c}{T2I gain} & \multicolumn{2}{c}{I2T gain} \\ & & R@1 & R@10 & R@1 & R@10 \\ \midrule
P0 & CLIP + place & +8.46 & \thirdresult{+24.63} & +7.54 & +23.19 \\
P0 & BLIP + MS & \bestresult{+13.46} & \bestresult{+31.17} & \bestresult{+19.21} & \bestresult{+36.76} \\
P0 & SigLIP2 + MS & \secondresult{+10.09} & \secondresult{+25.46} & \secondresult{+12.07} & \secondresult{+29.76} \\
P0 & SigLIP2 + place & \thirdresult{+8.79} & +24.10 & \thirdresult{+8.36} & \thirdresult{+25.51} \\
P1 & CLIP + place & +2.29 & \thirdresult{+9.14} & +1.90 & +7.81 \\
P1 & BLIP + MS & \bestresult{+4.95} & \bestresult{+14.69} & \bestresult{+7.26} & \bestresult{+19.47} \\
P1 & SigLIP2 + MS & \secondresult{+2.90} & \secondresult{+9.61} & \secondresult{+3.75} & \secondresult{+12.81} \\
P1 & SigLIP2 + place & \thirdresult{+2.48} & +8.51 & \thirdresult{+2.04} & \thirdresult{+9.29} \\
\bottomrule
\end{tabular}\par}

\paragraph{Interpretation.}
All four recipes improve the tested coarse references, but the gain varies with direction and retrieval cutoff. BLIP+MS yields a particularly strong coarse operating point in both protocols; this is evidence about the tested common-budget recipe, not a native-schedule reproduction. An increase at R@10 reflects broader candidate coverage and need not imply the same increase at R@1. The full-gallery P0--P1 comparison changes training cohorts, query identities, and gallery composition simultaneously; gains within a protocol are more directly interpretable than comparing raw percentages across protocols.

\end{minipage}}
\typeout{SUPPLEMENT-PANEL-2-HEIGHT: \the\dimexpr\ht\suppcontentbox+\dp\suppcontentbox\relax}
\noindent\makebox[\columnwidth][l]{\usebox{\suppcontentbox}}\par

\clearpage
\sbox{\suppcontentbox}{%
\begin{minipage}[t]{\textwidth}
\section{Reranking Responses and Directional Asymmetry}

\paragraph{Frozen systems can respond differently to the same reranker.}
The reranker is the already validation-selected BLIP ITM fusion stage. We compute selected-system minus coarse recall without selecting a different branch on test. Positive and negative cells therefore characterize fixed outputs; they are not a new tuning search.

\begin{center}
\includegraphics[width=.98\linewidth]{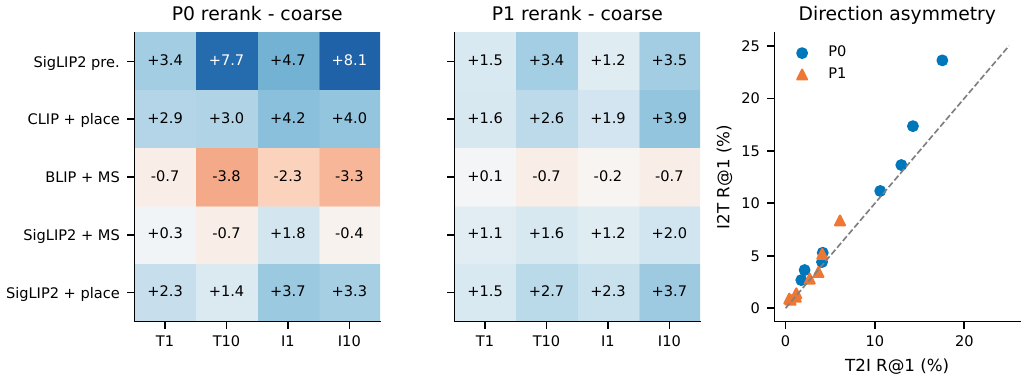}
\captionsetup{type=figure}
\caption{Left/middle: reranking changes in percentage points (T/I denote direction, 1/10 rank). Right: coarse T2I versus I2T R@1; the diagonal denotes equal directional recall.}
\end{center}

{\centering\small
\setlength{\tabcolsep}{4pt}
\captionsetup{type=table}
\caption{Reranking changes, in percentage points. A single validation-selected system can gain at one direction or cutoff and decline at another.}
\begin{tabular}{@{}llrrrr@{}}
\toprule
Protocol & Reference & T2I R@1 & T2I R@10 & I2T R@1 & I2T R@10 \\ \midrule
P0 & SigLIP2 pre. & \bestresult{+3.45} & \bestresult{+7.71} & \bestresult{+4.74} & \bestresult{+8.08} \\
P0 & CLIP + place & \secondresult{+2.95} & \secondresult{+3.00} & \secondresult{+4.21} & \secondresult{+3.98} \\
P0 & BLIP + MS & -0.68 & -3.78 & -2.34 & -3.33 \\
P0 & SigLIP2 + MS & +0.31 & -0.70 & +1.85 & -0.37 \\
P0 & SigLIP2 + place & \thirdresult{+2.29} & \thirdresult{+1.43} & \thirdresult{+3.71} & \thirdresult{+3.33} \\
P1 & SigLIP2 pre. & \secondresult{+1.54} & \bestresult{+3.37} & \thirdresult{+1.23} & \thirdresult{+3.50} \\
P1 & CLIP + place & \bestresult{+1.61} & \thirdresult{+2.63} & \secondresult{+1.88} & \bestresult{+3.92} \\
P1 & BLIP + MS & +0.14 & -0.66 & -0.19 & -0.69 \\
P1 & SigLIP2 + MS & +1.14 & +1.63 & +1.22 & +1.96 \\
P1 & SigLIP2 + place & \thirdresult{+1.53} & \secondresult{+2.73} & \bestresult{+2.26} & \secondresult{+3.67} \\
\bottomrule
\end{tabular}\par}

\paragraph{Representation-dependent effects.}
On P0, BLIP+MS changes by $-0.68$ points at T2I R@1 and $-2.34$ at I2T R@1; its R@10 also decreases in both directions. Other coarse references benefit more. The scatter illustrates that directional symmetry is not automatic even though both directions share the same place-ID relevance rule. Their query distributions and numbers of same-place gallery samples differ. Neither asymmetric recall nor a reranking decline identifies a unique failure mechanism: candidate coverage, similarity calibration, and cross-modal scoring can all contribute.

\end{minipage}}
\typeout{SUPPLEMENT-PANEL-3-HEIGHT: \the\dimexpr\ht\suppcontentbox+\dp\suppcontentbox\relax}
\noindent\makebox[\columnwidth][l]{\usebox{\suppcontentbox}}\par

\clearpage
\sbox{\suppcontentbox}{%
\begin{minipage}[t]{\textwidth}
\section{Adaptation Components Under the Same Protocol}

\paragraph{What this comparison controls.}
The SigLIP2 component variants retain the fixed protocol and the recorded common training budget. They train only residual heads, omit residual heads, adapt the vision tower alone, adapt the text tower alone, or adapt both towers with heads. This tests sensitivity to the chosen adaptation components. It does not introduce a new architecture, and changing the trainable parameter subset also changes optimization capacity.

\begin{center}
\includegraphics[width=.98\linewidth]{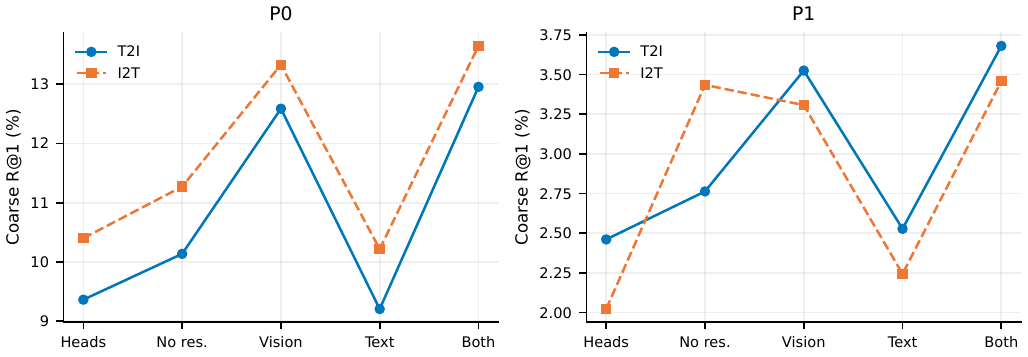}
\captionsetup{type=figure}
\caption{Coarse bidirectional R@1 across adaptation variants. The x-axis lists categorical configurations; connecting segments aid comparison rather than imply a continuous parameter sweep.}
\end{center}

{\centering\small
\setlength{\tabcolsep}{4pt}
\captionsetup{type=table}
\caption{Adaptation sensitivity in percent; mean $\pm$ sample SD across three training seeds.}
\begin{tabular}{@{}llrrrr@{}}
\toprule
Protocol & Variant & \multicolumn{2}{c}{Coarse R@1} & \multicolumn{2}{c}{Reranked R@1} \\ & & T2I & I2T & T2I & I2T \\ \midrule
P0 & Heads only & 9.36 $\pm$ 0.10 & 10.40 $\pm$ 0.18 & 12.31 $\pm$ 0.67 & 15.06 $\pm$ 0.53 \\
P0 & No residual heads & \thirdresult{10.14 $\pm$ 0.16} & \thirdresult{11.27 $\pm$ 0.10} & 13.09 $\pm$ 0.07 & \thirdresult{15.47 $\pm$ 0.21} \\
P0 & Vision only & \secondresult{12.59 $\pm$ 0.21} & \secondresult{13.33 $\pm$ 0.19} & \secondresult{15.01 $\pm$ 0.07} & \bestresult{17.47 $\pm$ 0.10} \\
P0 & Text only & 9.21 $\pm$ 0.18 & 10.22 $\pm$ 0.34 & \thirdresult{13.15 $\pm$ 0.76} & 15.39 $\pm$ 0.49 \\
P0 & Both + heads & \bestresult{12.95 $\pm$ 0.22} & \bestresult{13.64 $\pm$ 0.27} & \bestresult{15.24 $\pm$ 0.30} & \secondresult{17.35 $\pm$ 0.15} \\
P1 & Heads only & 2.46 $\pm$ 0.04 & 2.02 $\pm$ 0.11 & 4.08 $\pm$ 0.02 & 4.16 $\pm$ 0.02 \\
P1 & No residual heads & \thirdresult{2.76 $\pm$ 0.03} & \secondresult{3.43 $\pm$ 0.06} & \thirdresult{4.53 $\pm$ 0.04} & \thirdresult{5.00 $\pm$ 0.04} \\
P1 & Vision only & \secondresult{3.52 $\pm$ 0.05} & \thirdresult{3.31 $\pm$ 0.04} & \secondresult{5.13 $\pm$ 0.03} & \secondresult{5.41 $\pm$ 0.01} \\
P1 & Text only & 2.53 $\pm$ 0.04 & 2.24 $\pm$ 0.11 & 4.16 $\pm$ 0.00 & 4.51 $\pm$ 0.06 \\
P1 & Both + heads & \bestresult{3.68 $\pm$ 0.05} & \bestresult{3.46 $\pm$ 0.04} & \bestresult{5.21 $\pm$ 0.05} & \bestresult{5.72 $\pm$ 0.08} \\
\bottomrule
\end{tabular}\par}

\paragraph{Why the scoring stage matters.}
The component ranking should be assessed separately for coarse retrieval and the frozen reranked system. An adaptation that alters candidate coverage can interact with the reranker even when its coarse R@1 changes little. The table preserves both outputs instead of selecting the better one after testing. All variants are finite-budget references; a weaker result here is not evidence that a component can never help under a different training schedule. The benchmark interpretation remains the same: place supervision can improve representations while leaving substantial dependence on observation and gallery conditions.

\end{minipage}}
\typeout{SUPPLEMENT-PANEL-4-HEIGHT: \the\dimexpr\ht\suppcontentbox+\dp\suppcontentbox\relax}
\noindent\makebox[\columnwidth][l]{\usebox{\suppcontentbox}}\par

\clearpage
\sbox{\suppcontentbox}{%
\begin{minipage}[t]{\textwidth}
\section{Training-Seed Dispersion and Checkpoint Selection}

\paragraph{Reported variation is training variation.}
Each supervised recipe uses seeds 42, 43, and 44. Error bars are sample SD over these three fitted systems, not confidence intervals over test queries. A small bar describes repeatability under this specific recipe and fixed dataset; it does not cover data resampling, annotation uncertainty, or an unseen geographic distribution.

\begin{center}
\includegraphics[width=.98\linewidth]{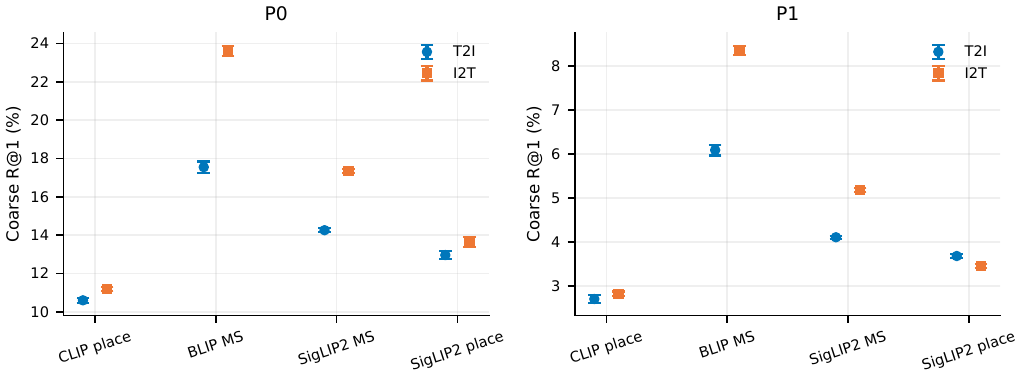}
\captionsetup{type=figure}
\caption{Coarse R@1 means and training-seed SD. Circle/square markers distinguish T2I and I2T.}
\end{center}

{\centering\small
\setlength{\tabcolsep}{4pt}
\captionsetup{type=table}
\caption{Seed stability of the four supervised references. Epochs are the archived validation-selected coarse checkpoints.}
\begin{tabular}{@{}llrrrrl@{}}
\toprule
Protocol & Recipe & \multicolumn{2}{c}{T2I R@1} & \multicolumn{2}{c}{I2T R@1} & Selected epochs \\ & & Mean & SD & Mean & SD & Seeds 42/43/44 \\ \midrule
P0 & CLIP + place & 10.59 & 0.12 & 11.17 & 0.11 & 3,3,3 \\
P0 & BLIP + MS & \bestresult{17.54} & 0.30 & \bestresult{23.62} & 0.27 & 3,3,3 \\
P0 & SigLIP2 + MS & \secondresult{14.25} & 0.11 & \secondresult{17.35} & 0.09 & 3,3,3 \\
P0 & SigLIP2 + place & \thirdresult{12.95} & 0.22 & \thirdresult{13.64} & 0.27 & 3,3,3 \\
P1 & CLIP + place & 2.70 & 0.08 & 2.82 & 0.05 & 3,3,3 \\
P1 & BLIP + MS & \bestresult{6.09} & 0.12 & \bestresult{8.36} & 0.10 & 3,3,3 \\
P1 & SigLIP2 + MS & \secondresult{4.11} & 0.04 & \secondresult{5.18} & 0.04 & 3,3,3 \\
P1 & SigLIP2 + place & \thirdresult{3.68} & 0.05 & \thirdresult{3.46} & 0.04 & 3,3,3 \\
\bottomrule
\end{tabular}\par}

\paragraph{Selection is distinct from convergence.}
All listed coarse checkpoints were selected at epoch 3 under the recorded weaker-direction validation R@100 criterion. This shows that the final recorded epoch was preferred under that criterion; it does not establish that further training would be beneficial, harmful, or converged. Several between-method differences exceed the displayed seed SD, but formal claims about model superiority would require an appropriate paired evaluation and a broader uncertainty design. No new seed is generated here, and no test score changes checkpoint selection.

\end{minipage}}
\typeout{SUPPLEMENT-PANEL-5-HEIGHT: \the\dimexpr\ht\suppcontentbox+\dp\suppcontentbox\relax}
\noindent\makebox[\columnwidth][l]{\usebox{\suppcontentbox}}\par

\clearpage
\sbox{\suppcontentbox}{%
\begin{minipage}[t]{\textwidth}
\section{Epoch-Wise Optimization and Diminishing Increments}

\paragraph{Validation trajectories, not test trajectories.}
The eight panels expose the logged three-epoch budget. Loss values belong to different objectives and are not comparable as a quality ranking. Validation R@1 characterizes early candidate ranking; weaker-direction R@100 is the selection criterion and can improve without a matching change in every R@1 direction.

\begin{center}
\includegraphics[width=.88\linewidth]{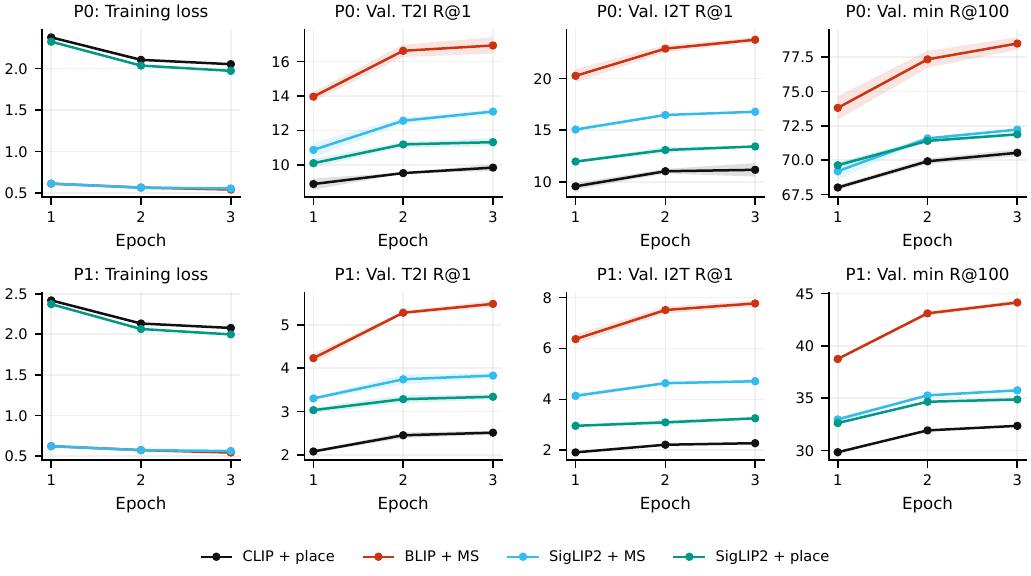}
\captionsetup{type=figure}
\caption{Three-seed means and SD across the logged training epochs; no epoch-zero measurements are invented.}
\end{center}

{\centering\small
\setlength{\tabcolsep}{4pt}
\captionsetup{type=table}
\caption{Changes in mean validation recall, in percentage points. These are not selected-checkpoint test gains.}
\begin{tabular}{@{}llrrrr@{}}
\toprule
Protocol & Recipe & \multicolumn{2}{c}{T2I R@1 increment} & \multicolumn{2}{c}{I2T R@1 increment} \\ & & 1 to 2 & 2 to 3 & 1 to 2 & 2 to 3 \\ \midrule
P0 & CLIP + place & +0.64 & \secondresult{+0.32} & \secondresult{+1.46} & +0.14 \\
P0 & BLIP + MS & \bestresult{+2.67} & \thirdresult{+0.31} & \bestresult{+2.63} & \bestresult{+0.86} \\
P0 & SigLIP2 + MS & \secondresult{+1.69} & \bestresult{+0.53} & \thirdresult{+1.41} & \thirdresult{+0.31} \\
P0 & SigLIP2 + place & \thirdresult{+1.09} & +0.13 & +1.12 & \secondresult{+0.34} \\
P1 & CLIP + place & \thirdresult{+0.37} & \thirdresult{+0.06} & \thirdresult{+0.30} & +0.06 \\
P1 & BLIP + MS & \bestresult{+1.05} & \bestresult{+0.20} & \bestresult{+1.14} & \bestresult{+0.26} \\
P1 & SigLIP2 + MS & \secondresult{+0.44} & \secondresult{+0.09} & \secondresult{+0.50} & \thirdresult{+0.07} \\
P1 & SigLIP2 + place & +0.25 & \thirdresult{+0.06} & +0.14 & \secondresult{+0.16} \\
\bottomrule
\end{tabular}\par}

\paragraph{What the plateau does and does not show.}
Every listed recipe improves mean bidirectional validation R@1 between epochs 1 and 3, while the later increment is often smaller. This supports reporting the training budget explicitly rather than describing these references as converged. It also explains why low training loss alone is not a stopping criterion for the benchmark. Longer schedules, different learning rates, or additional data remain untested hypotheses; the archived test set is not used to choose such changes.

\end{minipage}}
\typeout{SUPPLEMENT-PANEL-6-HEIGHT: \the\dimexpr\ht\suppcontentbox+\dp\suppcontentbox\relax}
\noindent\makebox[\columnwidth][l]{\usebox{\suppcontentbox}}\par

\clearpage
\sbox{\suppcontentbox}{%
\begin{minipage}[t]{\textwidth}
\section{Paired Observation Transfer as Hit Transitions}

\paragraph{Aggregate recall hides different transitions.}
For each paired place, a source-view hit can remain a hit, be lost, or be replaced by a new target-view hit that did not occur for the source. We average these transition fractions over the frozen training seeds. Pretrained controls have one frozen model. The same place is not counted as three independent observations merely because three checkpoints evaluate it.

\begin{center}
\includegraphics[width=.98\linewidth]{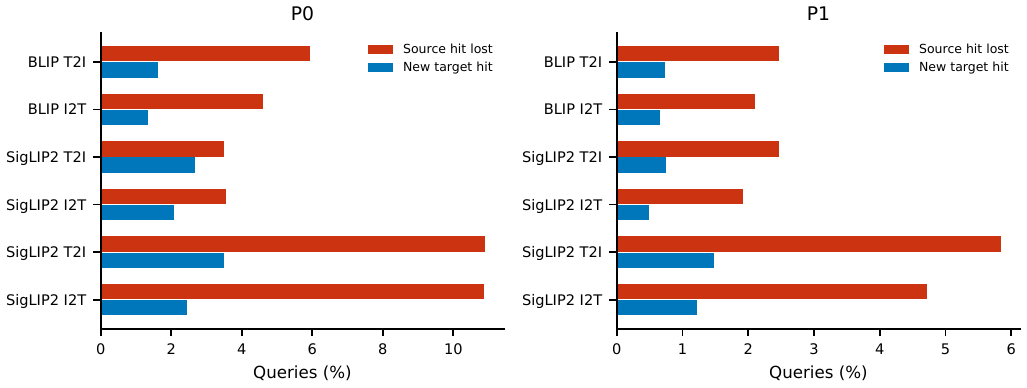}
\captionsetup{type=figure}
\caption{Percent of paired queries that lose a source-view R@1 hit or gain a new target-view hit. Each protocol has its own fixed singleton cohort.}
\end{center}

{\centering\small
\setlength{\tabcolsep}{4pt}
\captionsetup{type=table}
\caption{R@1 transitions. Shared misses complete each directional distribution to 100\%; counts are averaged over seeds where applicable.}
\begin{tabular}{@{}llrrrrrr@{}}
\toprule
Protocol & Reference & \multicolumn{3}{c}{T2I queries (\%)} & \multicolumn{3}{c}{I2T queries (\%)} \\ & & Both hit & Lost & New & Both hit & Lost & New \\ \midrule
P0 & BLIP pretrained & 1.85 & 5.93 & 1.63 & 2.30 & 4.60 & 1.33 \\
P0 & SigLIP2 pretrained & 2.22 & 3.48 & 2.67 & 2.52 & 3.56 & 2.08 \\
P0 & SigLIP2 supervised & 8.80 & 10.90 & 3.51 & 7.86 & 10.87 & 2.45 \\
P1 & BLIP pretrained & 0.38 & 2.47 & 0.74 & 0.39 & 2.10 & 0.65 \\
P1 & SigLIP2 pretrained & 0.52 & 2.47 & 0.75 & 0.64 & 1.92 & 0.49 \\
P1 & SigLIP2 supervised & 1.64 & 5.84 & 1.47 & 1.63 & 4.72 & 1.22 \\
\bottomrule
\end{tabular}\par}

\paragraph{A net decrease is not universal per-place failure.}
For supervised SigLIP2 on P0, 10.90\% of T2I queries lose a source hit while 3.51\% gain a target hit, yielding the approximately 7.39-point net decline. On P1, the corresponding fractions are 5.84\% and 1.47\%. Some independent observations are therefore easier for a fixed representation even though aggregate transfer is worse. The experiment replaces visual observations; it does not identify whether a particular lost hit is caused by time, orientation, occlusion, or description visibility. Transition analysis complements the paired bootstrap intervals reported in the principal account.

\end{minipage}}
\typeout{SUPPLEMENT-PANEL-7-HEIGHT: \the\dimexpr\ht\suppcontentbox+\dp\suppcontentbox\relax}
\noindent\makebox[\columnwidth][l]{\usebox{\suppcontentbox}}\par

\clearpage
\sbox{\suppcontentbox}{%
\begin{minipage}[t]{\textwidth}
\section{City-Level Heterogeneity in Independent-Observation Retrieval}

\paragraph{The controlled unit remains a place.}
We group the paired diagnostic queries by city without changing any gallery or model. Each heatmap cell is mean target-view R@10 for that city's query places; negatives remain the complete diagnostic pool for the protocol. B, S, and A denote pretrained BLIP, pretrained SigLIP2, and adapted SigLIP2; T/I denote retrieval direction. City labels include query counts.

\begin{center}
\includegraphics[width=.94\linewidth]{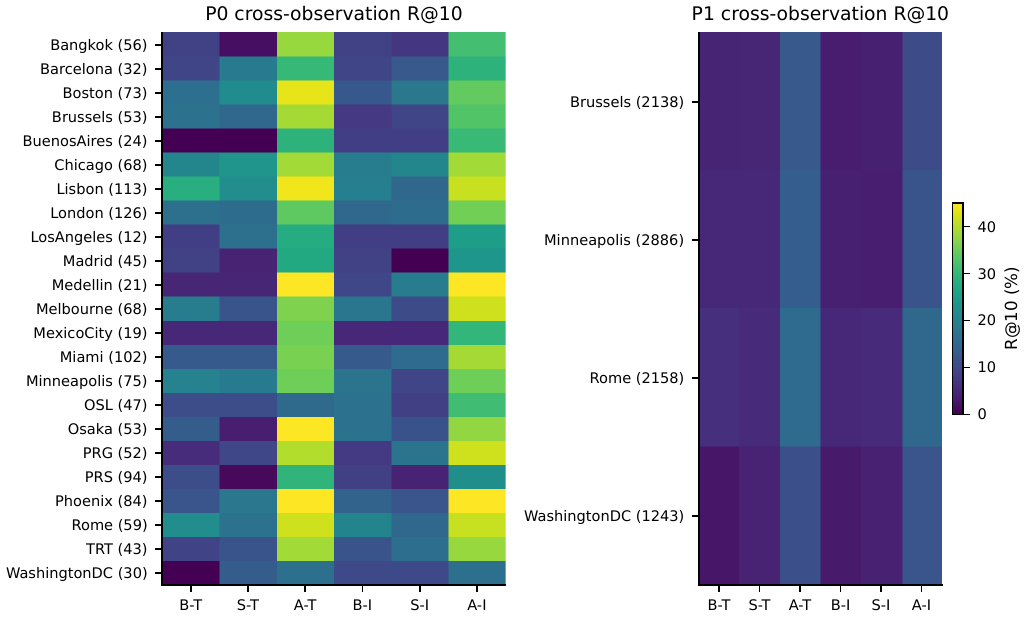}
\captionsetup{type=figure}
\caption{Per-city diagnostic R@10 (\%). P0 has 23 city groups; P1 has four held-out test cities. The common color scale is clipped at 45\% for visual contrast; machine-readable values retain values above this limit.}
\end{center}

{\centering\small
\setlength{\tabcolsep}{4pt}
\captionsetup{type=table}
\caption{Adapted SigLIP2 macro/micro summaries. Macro gives each city equal weight; micro weights cities by their query counts.}
\begin{tabular}{@{}llrrr@{}}
\toprule
Protocol & Direction & Cities & City-macro R@10 & Query-micro R@10 \\ \midrule
P0 & T2I & 23 & 35.76 & 36.84 \\
P0 & I2T & 23 & 34.30 & 35.53 \\
P1 & T2I & 4 & 13.19 & 13.44 \\
P1 & I2T & 4 & 12.26 & 12.27 \\
\bottomrule
\end{tabular}\par}

\paragraph{Composition changes the summary.}
In P0, adapted T2I R@10 ranges from 15.60\% in OSL to 51.57\% in Osaka; these groups contain 47 and 53 queries. P1 ranges from 11.05\% in WashingtonDC to 15.79\% in Rome, with much larger groups. Such heterogeneity motivates reporting sample counts and aggregation rules. The city differences combine visual content, descriptions, available captures, and competition from other places. They are not causal estimates of geographic difficulty, nor are small P0 groups reliable rankings of cities. No city-specific tuning is performed.

\end{minipage}}
\typeout{SUPPLEMENT-PANEL-8-HEIGHT: \the\dimexpr\ht\suppcontentbox+\dp\suppcontentbox\relax}
\noindent\makebox[\columnwidth][l]{\usebox{\suppcontentbox}}\par

\clearpage
\sbox{\suppcontentbox}{%
\begin{minipage}[t]{\textwidth}
\section{Capture-Time and Heading Metadata}

\paragraph{Independent observations are not uniformly extreme viewpoints.}
We derive circular heading gaps in $[0,180]$ degrees and absolute month gaps from the selected source/target metadata. The empirical distributions describe the same paired diagnostic cohort used for observation transfer. Heading is a capture attribute, not a measurement of visible overlap or landmark visibility.

\begin{center}
\includegraphics[width=.92\linewidth]{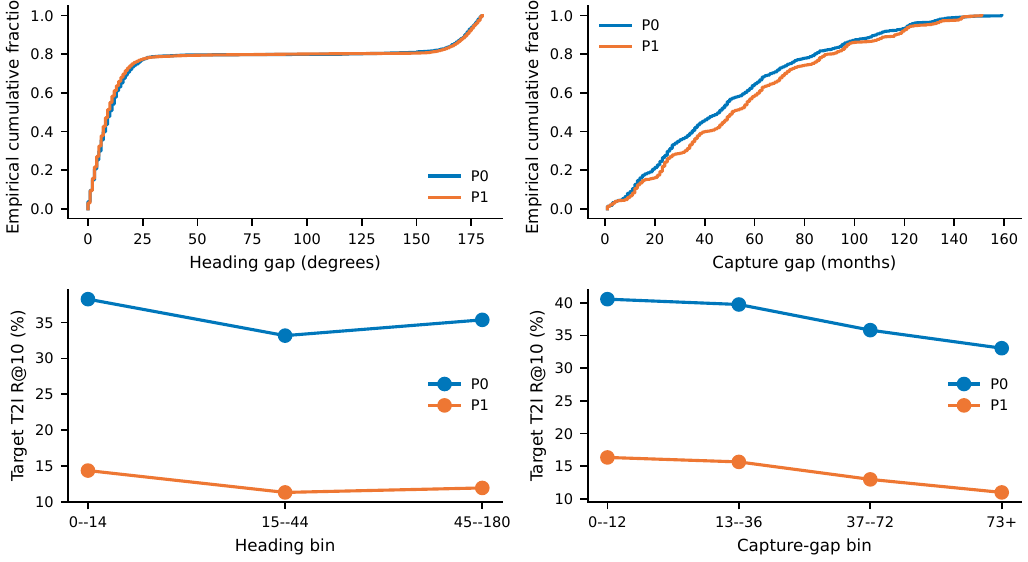}
\captionsetup{type=figure}
\caption{Top: metadata distributions. Bottom: adapted target T2I R@10 by metadata bin; bins are post-hoc descriptive groups, not controlled interventions.}
\end{center}

{\centering\small
\setlength{\tabcolsep}{4pt}
\captionsetup{type=table}
\caption{Capture-gap quantiles for selected paired observations. Heading is in degrees; capture gap is in months.}
\begin{tabular}{@{}llrrrr@{}}
\toprule
Protocol & Metadata & 25th & Median & 75th & 90th \\ \midrule
P0 & Heading (degrees) & 4.00 & 10.00 & 23.00 & 172.00 \\
P0 & Capture gap (months) & 23.00 & 46.00 & 74.00 & 109.00 \\
P1 & Heading (degrees) & 4.00 & 9.00 & 21.00 & 173.00 \\
P1 & Capture gap (months) & 25.00 & 51.00 & 83.00 & 116.00 \\
\bottomrule
\end{tabular}\par}

\paragraph{Temporal association is visible, but confounded.}
For P1, target T2I R@10 is 16.35\% in the 0--12 month group and 11.00\% for gaps of at least 73 months; P0 shows 40.55\% and 33.05\%. The heading relation is not monotonic across all bins: P0 obtains 38.27\%, 33.18\%, and 35.39\% for gaps below 15, 15--44, and at least 45 degrees. These associations are consistent with several explanations, including scene persistence and place composition. They do not isolate temporal robustness or angular invariance. Bin counts and exact scores are preserved in the released capture-diagnostic JSON; no pair is removed because of its retrieval outcome.

\end{minipage}}
\typeout{SUPPLEMENT-PANEL-9-HEIGHT: \the\dimexpr\ht\suppcontentbox+\dp\suppcontentbox\relax}
\noindent\makebox[\columnwidth][l]{\usebox{\suppcontentbox}}\par

\clearpage
\sbox{\suppcontentbox}{%
\begin{minipage}[t]{\textwidth}
\section{Caption Length and Generation-Type Associations}

\paragraph{A selected-caption analysis.}
This analysis uses only the valid, single-source descriptions selected for the paired diagnostic. Length is the number of whitespace-delimited tokens, not a tokenizer-specific sequence length. We retain the original description text and generation type; no caption is edited or lengthened. The four length bins are post-hoc groups, and some groups are much smaller than others.

\begin{center}
\includegraphics[width=.90\linewidth]{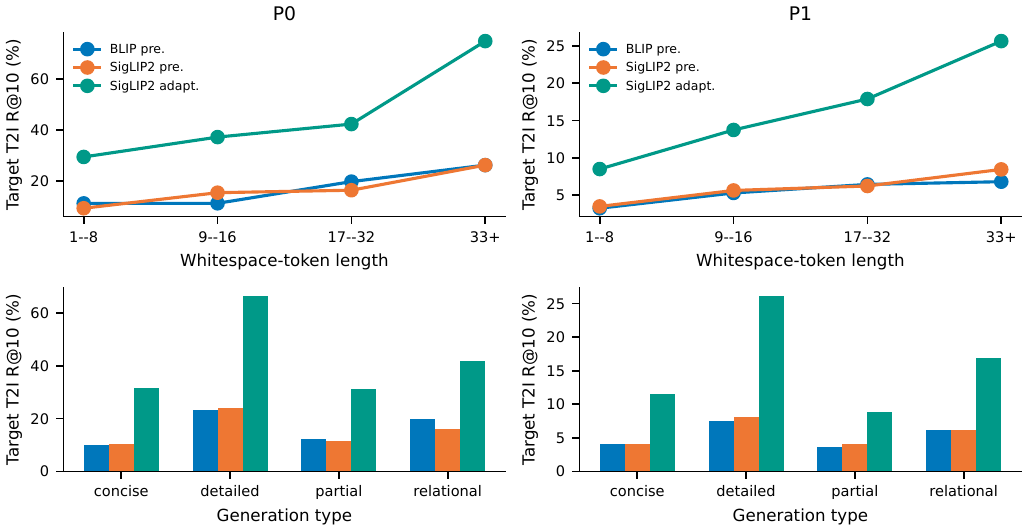}
\captionsetup{type=figure}
\caption{Target T2I R@10 by caption length (top) and categorical generation type (bottom), within each fixed diagnostic protocol. Type and length are associated and are not independent controls.}
\end{center}

{\centering\small
\setlength{\tabcolsep}{4pt}
\captionsetup{type=table}
\caption{Selected-description length groups, in percent. Each place contributes one paired-diagnostic caption.}
\begin{tabular}{@{}llrrr@{}}
\toprule
Protocol & Token bin & Places & Adapted T2I R@10 & Adapted I2T R@10 \\ \midrule
P0 & 1--8 & 633 & 29.44 & 30.96 \\
P0 & 9--16 & 240 & 37.22 & 34.31 \\
P0 & 17--32 & 415 & 42.33 & 39.76 \\
P0 & 33+ & 61 & 74.86 & 59.02 \\
P1 & 1--8 & 3698 & 8.52 & 7.71 \\
P1 & 9--16 & 1486 & 13.75 & 12.83 \\
P1 & 17--32 & 2816 & 17.90 & 17.00 \\
P1 & 33+ & 425 & 25.65 & 18.59 \\
\bottomrule
\end{tabular}\par}

\paragraph{Additional words are not a causal treatment.}
P1 adapted T2I R@10 increases from 8.52\% for 1--8 tokens to 25.65\% for 33 or more; P0 increases from 29.44\% to 74.86\%. The latter long-caption group has only 61 places, compared with 633 short-caption places. Longer captions can encode more distinguishing facts, but length also co-varies with generation type, source evidence, and scene content. These observations cannot justify automatically maximizing caption length, and they are not a length-controlled benchmark ranking. A future intervention would need paired edits on the same places while preserving correctness and target visibility.

\end{minipage}}
\typeout{SUPPLEMENT-PANEL-10-HEIGHT: \the\dimexpr\ht\suppcontentbox+\dp\suppcontentbox\relax}
\noindent\makebox[\columnwidth][l]{\usebox{\suppcontentbox}}\par

\clearpage
\sbox{\suppcontentbox}{%
\begin{minipage}[t]{\textwidth}
\section{Fixed-Query Gallery Scaling and Endpoint Retention}

\paragraph{Negative competition changes while queries remain fixed.}
The nested-gallery experiment retains 500 query places and their positives in each protocol. The final P0 and P1 pools have different sizes, so endpoint-retention ratios summarize their respective recorded sweeps rather than a common geographic treatment. The one-image/one-caption candidate pools also differ from the principal full-sample galleries.

\begin{center}
\includegraphics[width=.86\linewidth]{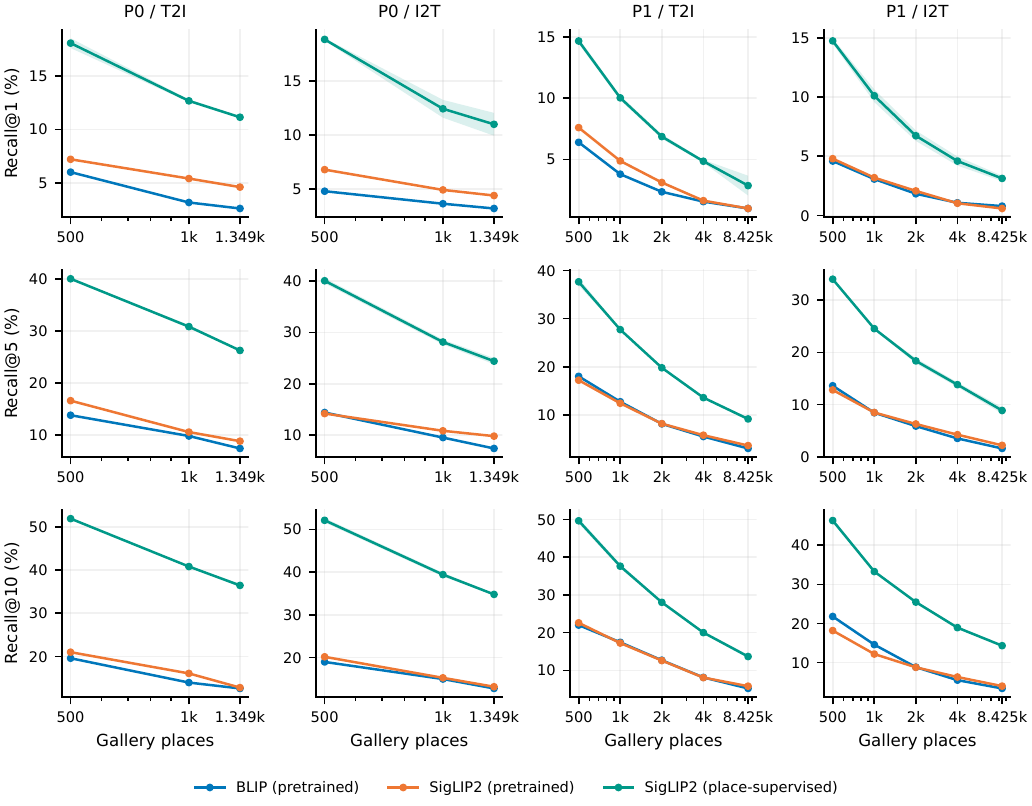}
\captionsetup{type=figure}
\caption{Gallery responses across protocol, direction, and cutoff. Points average nested-gallery samples within each checkpoint; adapted bands show training-seed SD. Full-pool repetitions are identical, not independent samples.}
\end{center}

{\centering\small
\setlength{\tabcolsep}{4pt}
\captionsetup{type=table}
\caption{Endpoint recall and final/initial retention. Final means 1,349 places for P0 and 8,425 for P1.}
\begin{tabular}{@{}llrrrrrr@{}}
\toprule
Protocol & Reference & \multicolumn{3}{c}{T2I R@1} & \multicolumn{3}{c}{I2T R@1} \\ & & 500 & Final & Retain\% & 500 & Final & Retain\% \\ \midrule
P0 & BLIP pretrained & \thirdresult{6.00} & \thirdresult{2.60} & 43.33 & \thirdresult{4.80} & \thirdresult{3.20} & 66.67 \\
P0 & SigLIP2 pretrained & \secondresult{7.20} & \secondresult{4.60} & 63.89 & \secondresult{6.80} & \secondresult{4.40} & 64.71 \\
P0 & SigLIP2 supervised & \bestresult{18.07} & \bestresult{11.13} & 61.62 & \bestresult{18.87} & \bestresult{11.00} & 58.30 \\
P1 & BLIP pretrained & \thirdresult{6.40} & \secondresult{1.00} & 15.62 & \thirdresult{4.60} & \secondresult{0.80} & 17.39 \\
P1 & SigLIP2 pretrained & \secondresult{7.60} & \secondresult{1.00} & 13.16 & \secondresult{4.80} & \thirdresult{0.60} & 12.50 \\
P1 & SigLIP2 supervised & \bestresult{14.67} & \bestresult{2.87} & 19.55 & \bestresult{14.73} & \bestresult{3.13} & 21.27 \\
\bottomrule
\end{tabular}\par}

\paragraph{Interpretation.}
Adapted P1 T2I recall retains about one fifth of its 500-place level at the full diagnostic pool. Rank-10 curves also decline, demonstrating that the effect is not confined to the first result. This design isolates candidate-pool expansion for fixed queries and weights; it does not show how a newly trained model would respond to a larger training dataset. The final fixed-query score must not be equated with recall over every eligible query place.

\end{minipage}}
\typeout{SUPPLEMENT-PANEL-11-HEIGHT: \the\dimexpr\ht\suppcontentbox+\dp\suppcontentbox\relax}
\noindent\makebox[\columnwidth][l]{\usebox{\suppcontentbox}}\par

\clearpage
\sbox{\suppcontentbox}{%
\begin{minipage}[t]{\textwidth}
\section{Gallery-Draw Variation at Matched Cardinality}

\paragraph{Five candidate draws are not five training runs.}
At 1,000 places, the diagnostic changes sampled candidates and associated queries according to the predefined gallery draws. Each pretrained checkpoint evaluates all five draws. For adapted SigLIP2, each of three training checkpoints evaluates the same five draws. The displayed points average training seeds within each draw; the table separately summarizes candidate-draw and training-seed variation.

\begin{center}
\includegraphics[width=.85\linewidth]{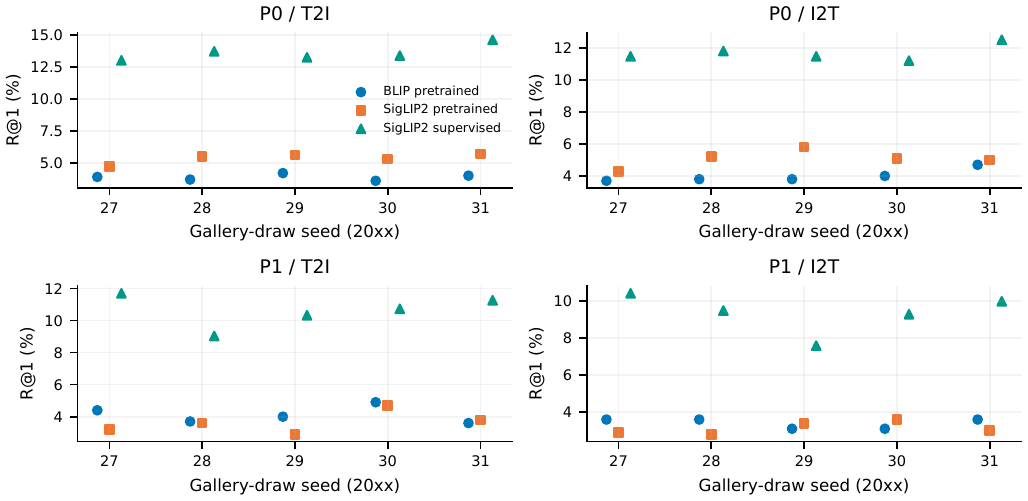}
\captionsetup{type=figure}
\caption{R@1 for five fixed 1,000-place draws. The x-axis is a categorical draw identifier, not a time or optimization variable.}
\end{center}

{\centering\small
\setlength{\tabcolsep}{4pt}
\captionsetup{type=table}
\caption{Draw SD is the five-draw sample SD per checkpoint, averaged over checkpoints. Seed SD uses each checkpoint\textquotesingle s five-draw mean. Values are percentage points.}
\begin{tabular}{@{}lllrrr@{}}
\toprule
Protocol & Reference & Direction & Mean R@1 & Draw SD & Seed SD \\ \midrule
P0 & BLIP pretrained & T2I & \thirdresult{3.88} & 0.24 & -- \\
P0 & SigLIP2 pretrained & T2I & \secondresult{5.36} & 0.40 & -- \\
P0 & SigLIP2 supervised & T2I & \bestresult{13.58} & 0.70 & 0.04 \\
P0 & BLIP pretrained & I2T & \thirdresult{4.00} & 0.41 & -- \\
P0 & SigLIP2 pretrained & I2T & \secondresult{5.08} & 0.54 & -- \\
P0 & SigLIP2 supervised & I2T & \bestresult{11.69} & 0.53 & 0.28 \\
P1 & BLIP pretrained & T2I & \secondresult{4.12} & 0.54 & -- \\
P1 & SigLIP2 pretrained & T2I & \thirdresult{3.64} & 0.69 & -- \\
P1 & SigLIP2 supervised & T2I & \bestresult{10.61} & 1.07 & 0.18 \\
P1 & BLIP pretrained & I2T & \secondresult{3.40} & 0.27 & -- \\
P1 & SigLIP2 pretrained & I2T & \thirdresult{3.14} & 0.34 & -- \\
P1 & SigLIP2 supervised & I2T & \bestresult{9.37} & 1.13 & 0.06 \\
\bottomrule
\end{tabular}\par}

\paragraph{A concrete separation of uncertainties.}
For adapted P0 T2I, mean R@1 is 13.58\%, mean within-checkpoint gallery-draw SD is 0.70 points, and the SD of checkpoint means is 0.04 points. Thus, candidate sampling can matter even when training-seed means are stable. Equalizing candidate count removes the large raw gallery-size difference, but does not equalize place content or training coverage. The residual protocol difference is therefore not a pure estimate of city shift. The descriptive SDs should not be pooled into a nominal sample of fifteen independent experiments.

\end{minipage}}
\typeout{SUPPLEMENT-PANEL-12-HEIGHT: \the\dimexpr\ht\suppcontentbox+\dp\suppcontentbox\relax}
\noindent\makebox[\columnwidth][l]{\usebox{\suppcontentbox}}\par

\clearpage
\sbox{\suppcontentbox}{%
\begin{minipage}[t]{\textwidth}
\section{Rule-Status Differences Before and After Matching}

\paragraph{Retrieval association and factual quality are separate.}
We contrast rule-valid and rule-uncertain descriptions first on 7,735 paired places, then on 4,291 places matched by generation type, source observation, and word-count bin. The query-place cohort and gallery construction are fixed within each setting. Matching changes which places qualify; comparing the two settings is not a randomized correction of all confounders.

\begin{center}
\includegraphics[width=.98\linewidth]{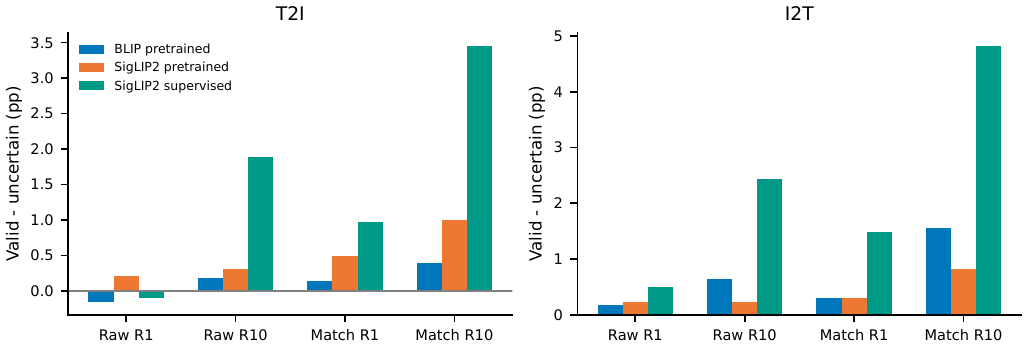}
\captionsetup{type=figure}
\caption{Valid-minus-uncertain differences at R@1 and R@10 for raw and matched P1 cohorts. Positive values favor valid captions in retrieval, without certifying their factual correctness.}
\end{center}

{\centering\small
\setlength{\tabcolsep}{4pt}
\captionsetup{type=table}
\caption{Absolute valid-minus-uncertain differences in percentage points; adapted results average three training seeds.}
\begin{tabular}{@{}llrrrr@{}}
\toprule
Reference & Cohort & \multicolumn{2}{c}{T2I gap} & \multicolumn{2}{c}{Controlled I2T gap} \\ & & R@1 & R@10 & R@1 & R@10 \\ \midrule
BLIP pretrained & Raw (7,735) & -0.16 & +0.18 & +0.18 & +0.65 \\
BLIP pretrained & Matched (4,291) & +0.14 & +0.40 & +0.30 & +1.56 \\
SigLIP2 pretrained & Raw (7,735) & +0.21 & +0.31 & +0.22 & +0.23 \\
SigLIP2 pretrained & Matched (4,291) & +0.49 & +1.00 & +0.30 & +0.82 \\
SigLIP2 supervised & Raw (7,735) & -0.09 & +1.89 & +0.50 & +2.44 \\
SigLIP2 supervised & Matched (4,291) & +0.97 & +3.46 & +1.48 & +4.82 \\
\bottomrule
\end{tabular}\par}

{\centering\small
\setlength{\tabcolsep}{4pt}
\captionsetup{type=table}
\caption{Absolute scores on the matched 4,291-place cohort; adapted values retain their archived seed SD.}
\begin{tabular}{@{}llrrrr@{}}
\toprule
Reference & Status & \multicolumn{2}{c}{T2I (\%)} & \multicolumn{2}{c}{Controlled I2T (\%)} \\ & & R@1 & R@10 & R@1 & R@10 \\ \midrule
BLIP (pretrained) & Valid & \thirdresult{1.19} & \thirdresult{4.47} & \thirdresult{0.86} & \secondresult{4.19} \\
BLIP (pretrained) & Uncertain & \secondresult{1.05} & \secondresult{4.08} & \thirdresult{0.56} & \thirdresult{2.63} \\
SigLIP2 (pretrained) & Valid & \secondresult{1.51} & \secondresult{4.85} & \secondresult{1.10} & \thirdresult{3.89} \\
SigLIP2 (pretrained) & Uncertain & \thirdresult{1.03} & \thirdresult{3.85} & \secondresult{0.79} & \secondresult{3.08} \\
SigLIP2 (place-supervised) & Valid & \bestresult{3.16 $\pm$ 0.14} & \bestresult{12.27 $\pm$ 0.16} & \bestresult{3.25 $\pm$ 0.21} & \bestresult{12.39 $\pm$ 0.36} \\
SigLIP2 (place-supervised) & Uncertain & \bestresult{2.19 $\pm$ 0.08} & \bestresult{8.81 $\pm$ 0.00} & \bestresult{1.78 $\pm$ 0.08} & \bestresult{7.57 $\pm$ 0.17} \\\bottomrule
\end{tabular}\par}

\paragraph{Matching changes the observed contrast.}
For adapted T2I R@1, the raw valid-minus-uncertain difference is approximately $-0.09$ points, whereas the matched difference is $+0.97$ points. At R@10 the matched T2I/I2T differences are $+3.46/+4.82$ points. This sensitivity demonstrates why an automatic status comparison must specify its cohort and controls. It does not reverse the human audit: rule status still lacks a certified factual-quality ordering. Residual content differences and screening rules remain possible explanations. P0 does not supply the corresponding uncertain-caption pool, so no unsupported P0 comparison is manufactured.

\end{minipage}}
\typeout{SUPPLEMENT-PANEL-13-HEIGHT: \the\dimexpr\ht\suppcontentbox+\dp\suppcontentbox\relax}
\noindent\makebox[\columnwidth][l]{\usebox{\suppcontentbox}}\par

\clearpage
\sbox{\suppcontentbox}{%
\begin{minipage}[t]{\textwidth}
\section{Joint Human Judgments and Rule-Stratum Composition}

\paragraph{The annotation axes are related measurements.}
The 240 audited descriptions receive source-correctness, target-visibility, and specificity labels from one blinded reviewer. Cross-tabulating the first two axes reveals how a correct source description can fail to transfer visually. Unknown labels are retained as separate outcomes. These counts neither estimate population prevalence nor provide inter-rater reliability.

\begin{center}
\includegraphics[width=.98\linewidth]{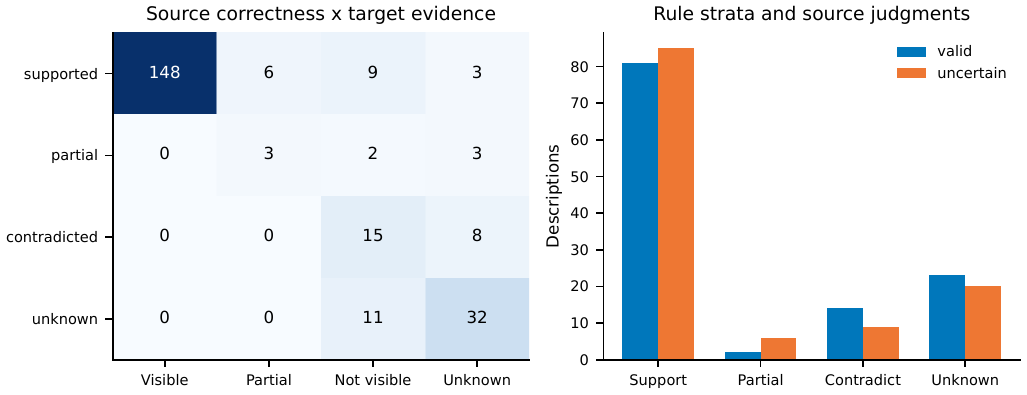}
\captionsetup{type=figure}
\caption{Joint source/target judgments and source-correctness counts by automatic rule stratum. Each rule stratum contains 120 descriptions.}
\end{center}

{\centering\small
\setlength{\tabcolsep}{4pt}
\captionsetup{type=table}
\caption{Observed joint human labels; the target columns concern the displayed target-image set, not every individual view.}
\begin{tabular}{@{}lrrrrr@{}}
\toprule
Source judgment & Visible & Partial & Not visible & Unknown & Total \\ \midrule
supported & 148 & 6 & 9 & 3 & 166 \\
partial & 0 & 3 & 2 & 3 & 8 \\
contradicted & 0 & 0 & 15 & 8 & 23 \\
unknown & 0 & 0 & 11 & 32 & 43 \\
\bottomrule
\end{tabular}\par}

\paragraph{What the joint pattern adds.}
All 148 target-visible descriptions in this reviewed sample are also fully source-supported. Of 166 source-supported descriptions, 18 are not fully target-visible: six are partial, nine not visible, and three unknown. The axes should therefore not be assumed statistically independent; the pattern may also reflect the related evidence and the single reviewer\textquotesingle s annotation logic. Source contradiction and target nonvisibility remain distinct judgments.

\paragraph{Screening labels do not replace this audit.}
Supported counts are 81 in the valid stratum and 85 in the uncertain stratum, while contradicted counts are 14 and nine. The balanced sampling and small groups preclude claiming that uncertain text is generally superior. The 240 rows cover 237 places, so row-level percentages are descriptive and should not be assigned independent-binomial population intervals without accounting for repeated places and stratified sampling.

\end{minipage}}
\typeout{SUPPLEMENT-PANEL-14-HEIGHT: \the\dimexpr\ht\suppcontentbox+\dp\suppcontentbox\relax}
\noindent\makebox[\columnwidth][l]{\usebox{\suppcontentbox}}\par

\clearpage
\sbox{\suppcontentbox}{%
\begin{minipage}[t]{\textwidth}
\section{Human-Stratified Retrieval Beyond a Single Cutoff}

\paragraph{Cutoff and annotation axis change the interpretation.}
We retain the audited query texts and the original frozen model outputs. The adapted reference averages three training seeds. T2I uses all 17,014 target-image candidates; controlled I2T replaces the focal caption in an 8,509-place, one-caption-per-place gallery and averages its two target-image query outcomes. These are diagnostic scores, not the principal all-description I2T leaderboard.

\begin{center}
\includegraphics[width=.90\linewidth]{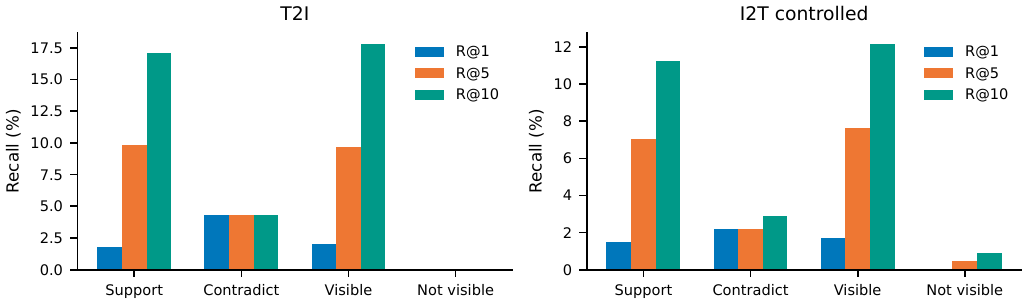}
\captionsetup{type=figure}
\caption{Adapted retrieval by source support and target visibility at three cutoffs. Groups overlap across annotation axes; bars do not denote independent cohorts.}
\end{center}

{\centering\small
\setlength{\tabcolsep}{4pt}
\captionsetup{type=table}
\caption{Percent recall for selected human groups; adapted results average three frozen training seeds.}
\begin{tabular}{@{}lrrrrrrr@{}}
\toprule
Human group & $n$ & \multicolumn{3}{c}{T2I} & \multicolumn{3}{c}{Controlled I2T} \\ & & R@1 & R@5 & R@10 & R@1 & R@5 & R@10 \\ \midrule
source correctness / supported & 166 & 1.81 & 9.84 & 17.07 & 1.51 & 7.03 & 11.24 \\
source correctness / contradicted & 23 & 4.35 & 4.35 & 4.35 & 2.17 & 2.17 & 2.90 \\
target visibility / visible & 148 & 2.03 & 9.68 & 17.79 & 1.69 & 7.66 & 12.16 \\
target visibility / not visible & 37 & 0.00 & 0.00 & 0.00 & 0.00 & 0.45 & 0.90 \\
target visibility / unknown & 46 & 2.17 & 2.17 & 2.17 & 1.09 & 1.81 & 2.90 \\
place specificity / distinctive & 133 & 2.26 & 10.78 & 19.80 & 1.88 & 8.52 & 13.66 \\
place specificity / generic & 42 & 2.38 & 2.38 & 2.38 & 1.19 & 1.19 & 1.59 \\
place specificity / unknown & 65 & 0.00 & 3.08 & 3.08 & 0.00 & 1.03 & 2.31 \\
\bottomrule
\end{tabular}\par}

{\centering\small
\setlength{\tabcolsep}{4pt}
\captionsetup{type=table}
\caption{Cross-model human-stratified R@10 (\%), retaining the earlier three-family comparison. I2T remains the controlled diagnostic.}
\begin{tabular}{@{}llrrrrrrr@{}}
\toprule
Axis & Judgment & $n$ & \multicolumn{2}{c}{BLIP pretrained} & \multicolumn{2}{c}{SigLIP2 pretrained} & \multicolumn{2}{c}{SigLIP2 adapted} \\ & & & T2I & I2T & T2I & I2T & T2I & I2T \\ \midrule
Source Correctness & supported & 166 & \secondresult{8.43} & \secondresult{7.83} & \thirdresult{4.82} & \thirdresult{3.61} & \bestresult{17.07} & \bestresult{11.24} \\
Source Correctness & contradicted & 23 & \secondresult{0.00} & \secondresult{2.17} & \secondresult{0.00} & \thirdresult{0.00} & \bestresult{4.35} & \bestresult{2.90} \\
Target Visibility & visible & 148 & \secondresult{8.78} & \secondresult{8.11} & \thirdresult{5.41} & \thirdresult{4.05} & \bestresult{17.79} & \bestresult{12.16} \\
Target Visibility & not visible & 37 & \bestresult{2.70} & \bestresult{2.70} & \secondresult{0.00} & \thirdresult{0.00} & \secondresult{0.00} & \secondresult{0.90} \\
Place Specificity & distinctive & 133 & \secondresult{9.77} & \secondresult{8.65} & \thirdresult{5.26} & \thirdresult{4.14} & \bestresult{19.80} & \bestresult{13.66} \\
Place Specificity & generic & 42 & \secondresult{0.00} & \secondresult{0.00} & \secondresult{0.00} & \secondresult{0.00} & \bestresult{2.38} & \bestresult{1.59} \\
Target Visibility & unknown & 46 & \secondresult{0.00} & \thirdresult{0.00} & \secondresult{0.00} & \secondresult{1.09} & \bestresult{2.17} & \bestresult{2.90} \\\bottomrule
\end{tabular}\par}

\paragraph{Rare hits should not dominate the scientific claim.}
The contradicted group has 23 items and can produce a higher R@1 percentage than the 166-item supported group from very few hits. At R@10, supported descriptions reach 17.07\% T2I versus 4.35\% for contradicted descriptions; visible descriptions reach 17.79\% versus 0\% for not-visible descriptions. This does not establish that correcting a caption would cause a particular retrieval improvement. Semantic content, specificity, and observability co-vary, and pair-level visibility does not certify each individual I2T query. The evidence supports distinguishing retrieval success from factual verification.

\end{minipage}}
\typeout{SUPPLEMENT-PANEL-15-HEIGHT: \the\dimexpr\ht\suppcontentbox+\dp\suppcontentbox\relax}
\noindent\makebox[\columnwidth][l]{\usebox{\suppcontentbox}}\par

\clearpage
\sbox{\suppcontentbox}{%
\begin{minipage}[t]{\textwidth}
\section{Shared Failures and Frozen-Model Complementarity}

\paragraph{A query-level overlap analysis.}
We compare the three model configurations for which the audited feature caches and exact rankings are available: pretrained BLIP, pretrained SigLIP2, and adapted SigLIP2 with seed 42. The supervised seed is fixed, not selected for qualitative performance. A binary pattern records which model obtains a place-ID hit at rank one. For I2T, this page uses the first target view, matching the visualized queries rather than the two-view average in the audit tables.

\begin{center}
\includegraphics[width=.98\linewidth]{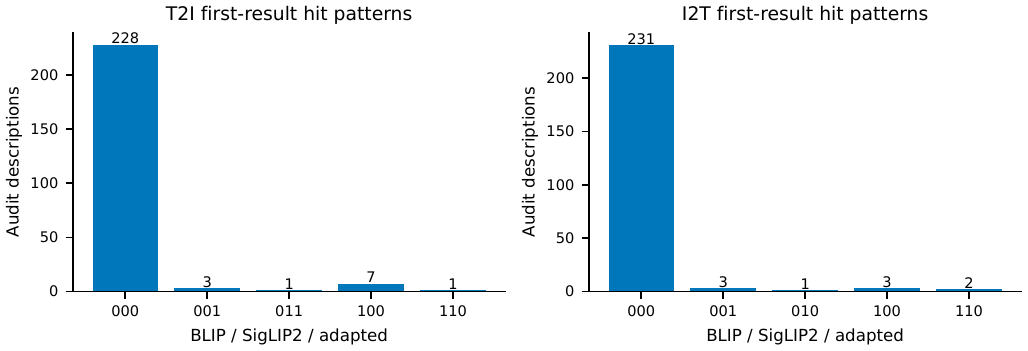}
\captionsetup{type=figure}
\caption{Observed R@1 success patterns among three frozen configurations on 240 audited descriptions. Most queries are shared misses; the audit is not a representative sample of all principal test queries.}
\end{center}

{\centering\small
\setlength{\tabcolsep}{4pt}
\captionsetup{type=table}
\caption{Numbers of audited descriptions with the indicated outcome. Union is a label-aware descriptive upper bound, not a deployed ensemble.}
\begin{tabular}{@{}lrrrrrr@{}}
\toprule
Direction & BLIP hits & SigLIP2 hits & Adapted hits & Union & Intersection & All miss \\ \midrule
T2I & \bestresult{8} & \thirdresult{2} & \secondresult{4} & 12 & 0 & 228 \\
I2T & \bestresult{5} & \secondresult{3} & \secondresult{3} & 9 & 0 & 231 \\
\bottomrule
\end{tabular}\par}

\paragraph{Complementarity exists within a difficult sample.}
For T2I, BLIP, SigLIP2, and the adapted model obtain eight, two, and four hits; their union contains 12 descriptions, while 228 are missed by all three. I2T has five, three, and three hits, a union of nine, and 231 shared misses. Neither direction contains a description hit by all three configurations. A hypothetical oracle that chooses a successful model after seeing relevance labels is not an inference-time retrieval method and must not be reported as a new benchmark result.

\paragraph{Scope limits.}
These outcomes do not contradict the full-gallery leaderboard: the human cohort includes uncertain captions and is deliberately balanced by rule status. It uses a different query distribution, and I2T uses the controlled replacement gallery. This analysis also does not include the stronger BLIP+MS adaptation or ITM reranked systems, whose audited feature caches are not available here. The useful conclusion is conditional: the inspected models have both shared failures and distinct successes, motivating analysis of evidence and competition rather than explaining every error through a single architectural weakness.

\end{minipage}}
\typeout{SUPPLEMENT-PANEL-16-HEIGHT: \the\dimexpr\ht\suppcontentbox+\dp\suppcontentbox\relax}
\noindent\makebox[\columnwidth][l]{\usebox{\suppcontentbox}}\par

\clearpage
\sbox{\suppcontentbox}{%
\begin{minipage}[t]{\textwidth}
\section{Qualitative Text-to-Image Retrieval}

\begin{center}
\includegraphics[width=.90\linewidth]{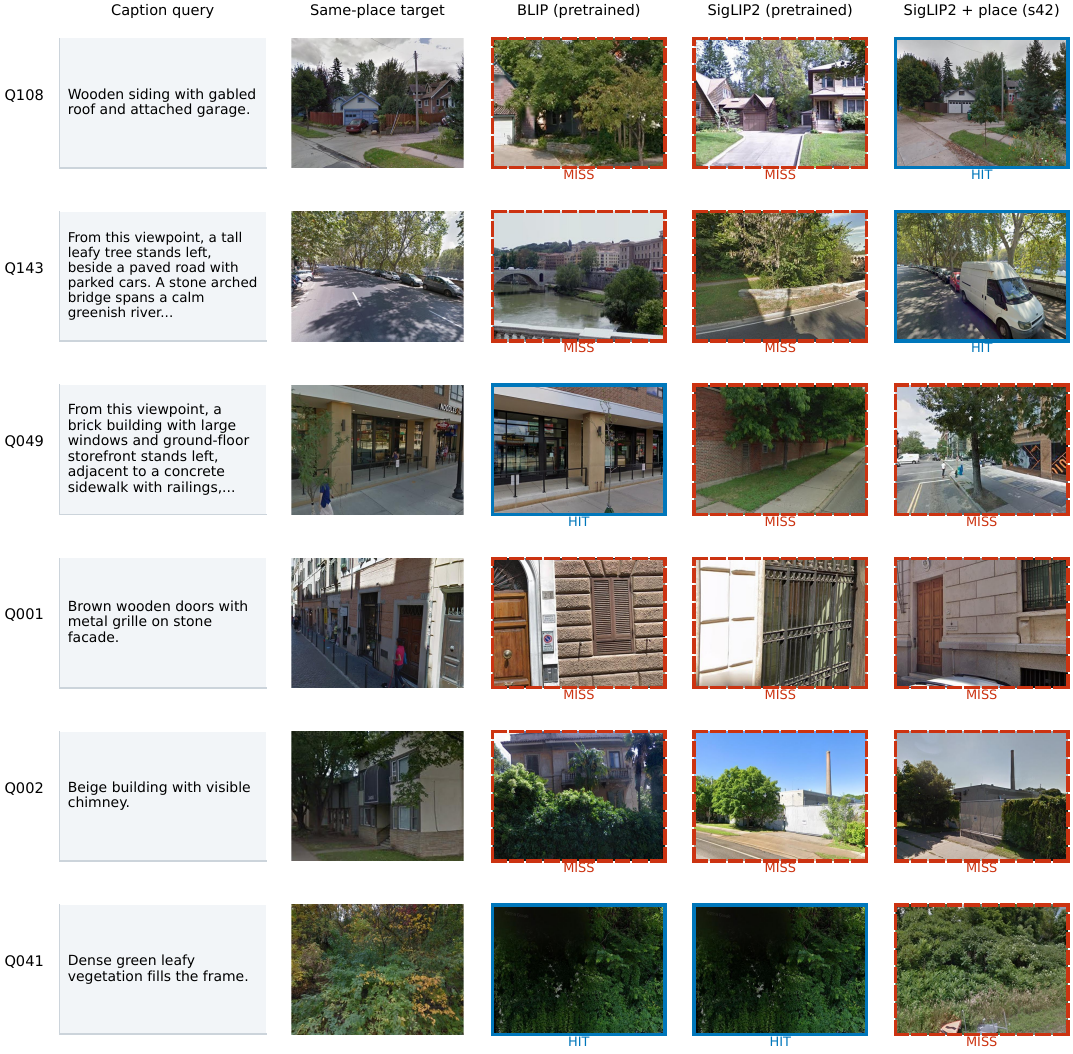}
\captionsetup{type=figure}
\caption{Six post-hoc T2I cases. Rows contain a caption query, one same-place target, and top-1 results from the full 17,014-image P1 gallery. Blue solid/HIT and red dashed/MISS encode place identity, not factual correctness.}
\end{center}

\paragraph{Reading the cases.}
Q108 and Q143 are adapted-only successes, Q049 is a BLIP-only success, and Q001/Q002 are shared failures. Q041 is hit by the two pretrained models but missed by the adapted model. Similar vegetation, entrances, or facade structure can generate plausible matches at the wrong place; the common miss pattern alone does not reveal which cue was used. The same-place reference shown is only one of multiple valid image positives. Cases were selected deterministically by audit ID within outcome strata, not randomly. They illustrate mechanisms and exceptions without estimating their frequency or selecting a preferred model. Complete captions, identities, and predictions remain available in the ranking records; ellipses denote display truncation.

\end{minipage}}
\typeout{SUPPLEMENT-PANEL-17-HEIGHT: \the\dimexpr\ht\suppcontentbox+\dp\suppcontentbox\relax}
\noindent\makebox[\columnwidth][l]{\usebox{\suppcontentbox}}\par

\clearpage
\sbox{\suppcontentbox}{%
\begin{minipage}[t]{\textwidth}
\section{Qualitative Image-to-Text Retrieval}

\begin{center}
\includegraphics[width=.90\linewidth]{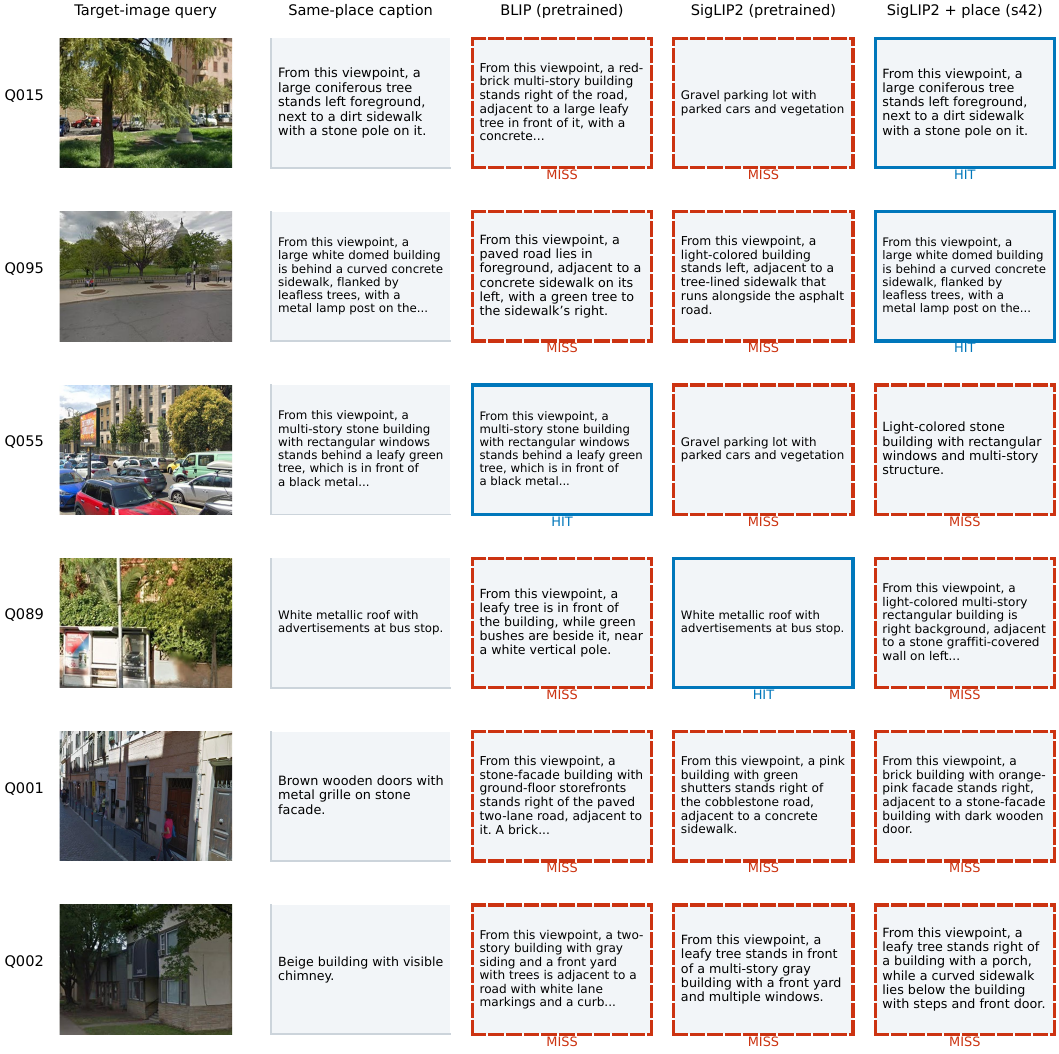}
\captionsetup{type=figure}
\caption{Six controlled I2T cases from an 8,509-caption replacement gallery. The first target view is shown; no ITM reranking is used. Same-place captions are stored annotations, not certified factual ground truth.}
\end{center}

\paragraph{Reading the cases.}
Q015/Q095 are adapted-only successes, Q055 favors pretrained BLIP, and Q089 favors pretrained SigLIP2; Q001/Q002 are shared failures. The opposite outcomes show that adaptation is not a per-query guarantee. A fluent returned description can remain wrong under place-ID relevance, while a place-ID hit does not establish that every sentence is visible in the query image. This page displays individual target queries; aggregate human I2T results average two views and should not be reconstructed from the six displayed rows. The same deterministic, post-hoc case-selection policy used for T2I is disclosed, and long display quotes are explicitly abbreviated. No model, fusion weight, caption, or gallery is changed to improve these examples.

\end{minipage}}
\typeout{SUPPLEMENT-PANEL-18-HEIGHT: \the\dimexpr\ht\suppcontentbox+\dp\suppcontentbox\relax}
\noindent\makebox[\columnwidth][l]{\usebox{\suppcontentbox}}\par
